# Supplementary material for: Gradient Cuff: Detecting Jailbreak Attacks on Large Language Models by Exploring Refusal Loss Landscapes
Source: arXiv:2403.00867 source file (2024-11-07)
Supplement: Supplementary file 2 [file trained_guards.tex]

\subsection{Comparison with Trained Guardrails}
\label{subapp:trained_guard}

{\color{red}While our main focus is on unsupervised methods as they do not require training a guardrail model to defend malicious queries, for completeness we perform comparisons to supervised methods. We compare our methods with LLaMA-Guard and Safe Decoding. The results are shown below:}

\input{tables/trained_guard}

{\color{red}We can summarize the experimental results as follows:
\begin{enumerate}[leftmargin=*]
   \item Safe-Decoding can achieve the largest average TPR against jailbreak attacks. But the FPR of Safe-Decoding is much higher which will bring unacceptable utility degradation.
    \item LLaMA-Guard can achieve comparable TPR results with Gradient Cuff on Vicuna-7B-V1.5 and a much lower TPR performance on LLaMA2-7B-Chat.
\end{enumerate}
}
{\color{red}
The experimental results showed that Gradient Cuff can also outperform these two baselines. Moreover, these supervised methods need to collect massive labelled data to train a guardrail model, while Gradient Cuff are training-free and only need to deploy the protected LLM itself in practice.
}
